# Supplementary material for: Text-based Sentiment Analysis and Music Emotion Recognition
Source: arXiv:1810.03031 source file (2018-10-06)
Supplement: Supplementary file 1 [file appendix2.tex]

% ******************************* Thesis Appendix B ********************************

\chapter{title of appendix}
